# Supplementary material for: Gaussian field model for polar fluids as a function of density and polarization: toward a model for water
Source: arXiv:1711.02541 source file (2017-11-07)

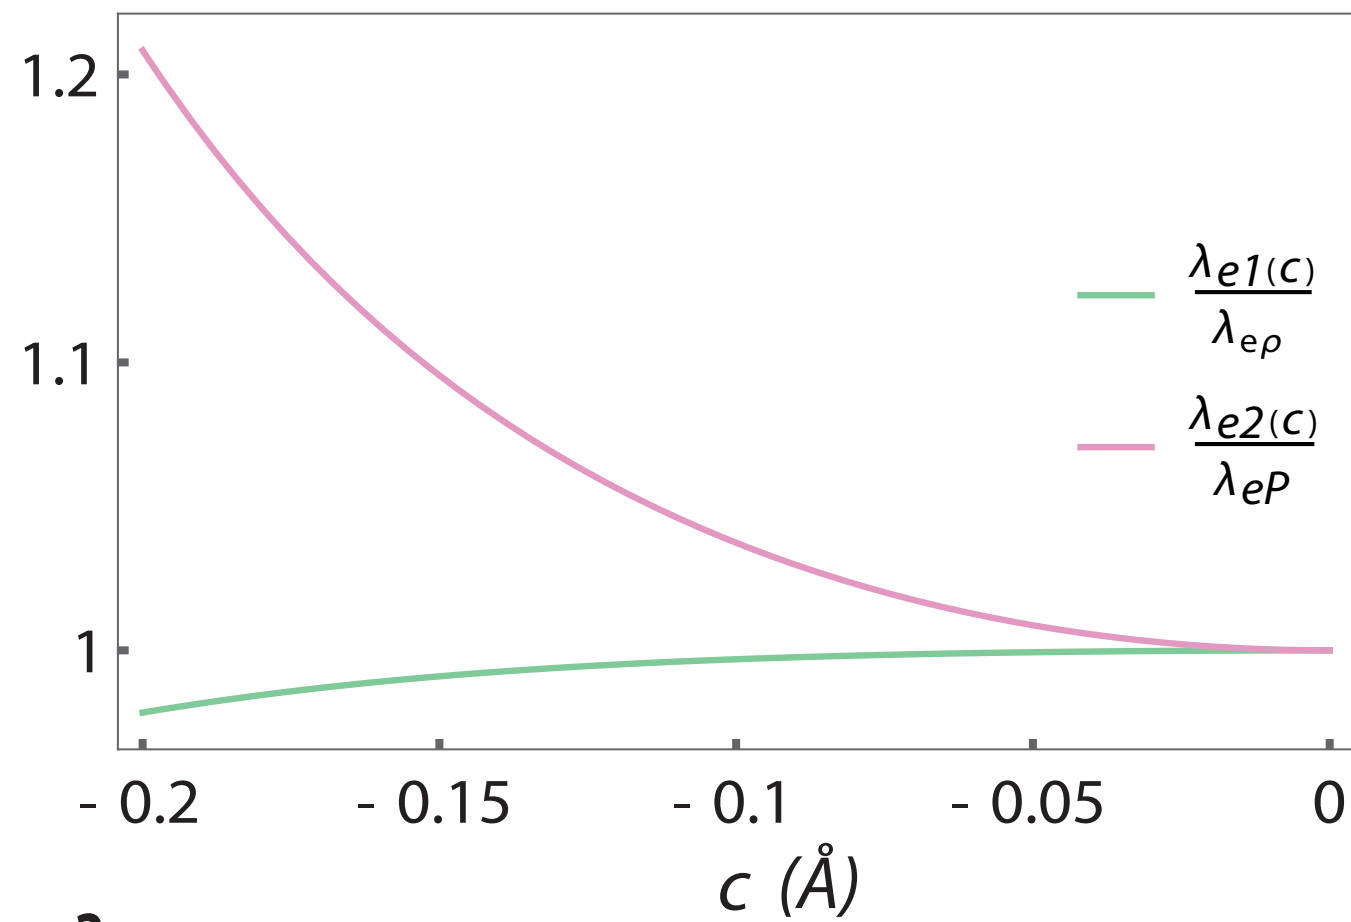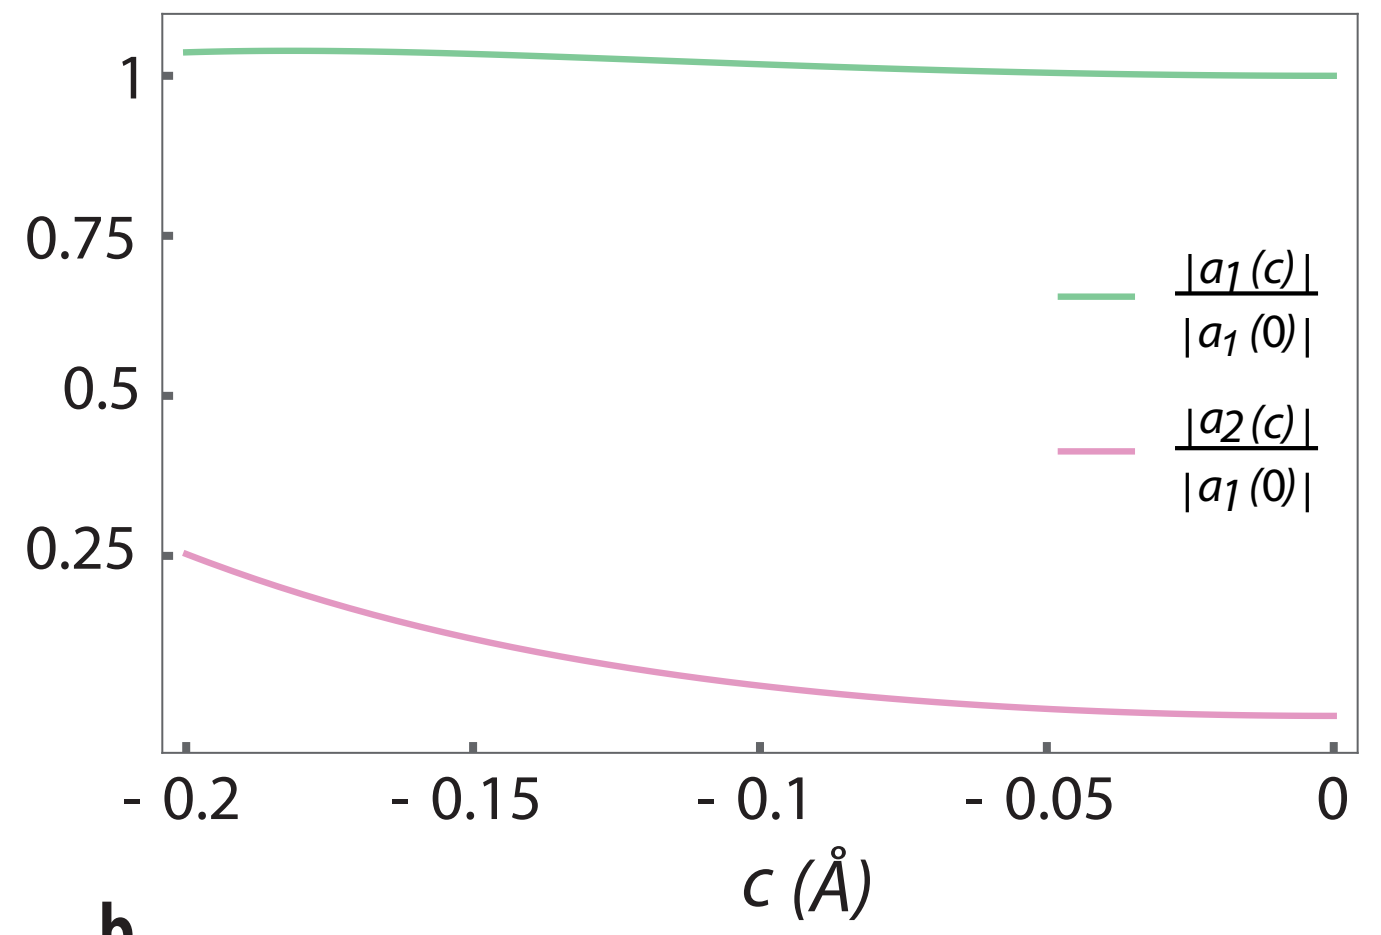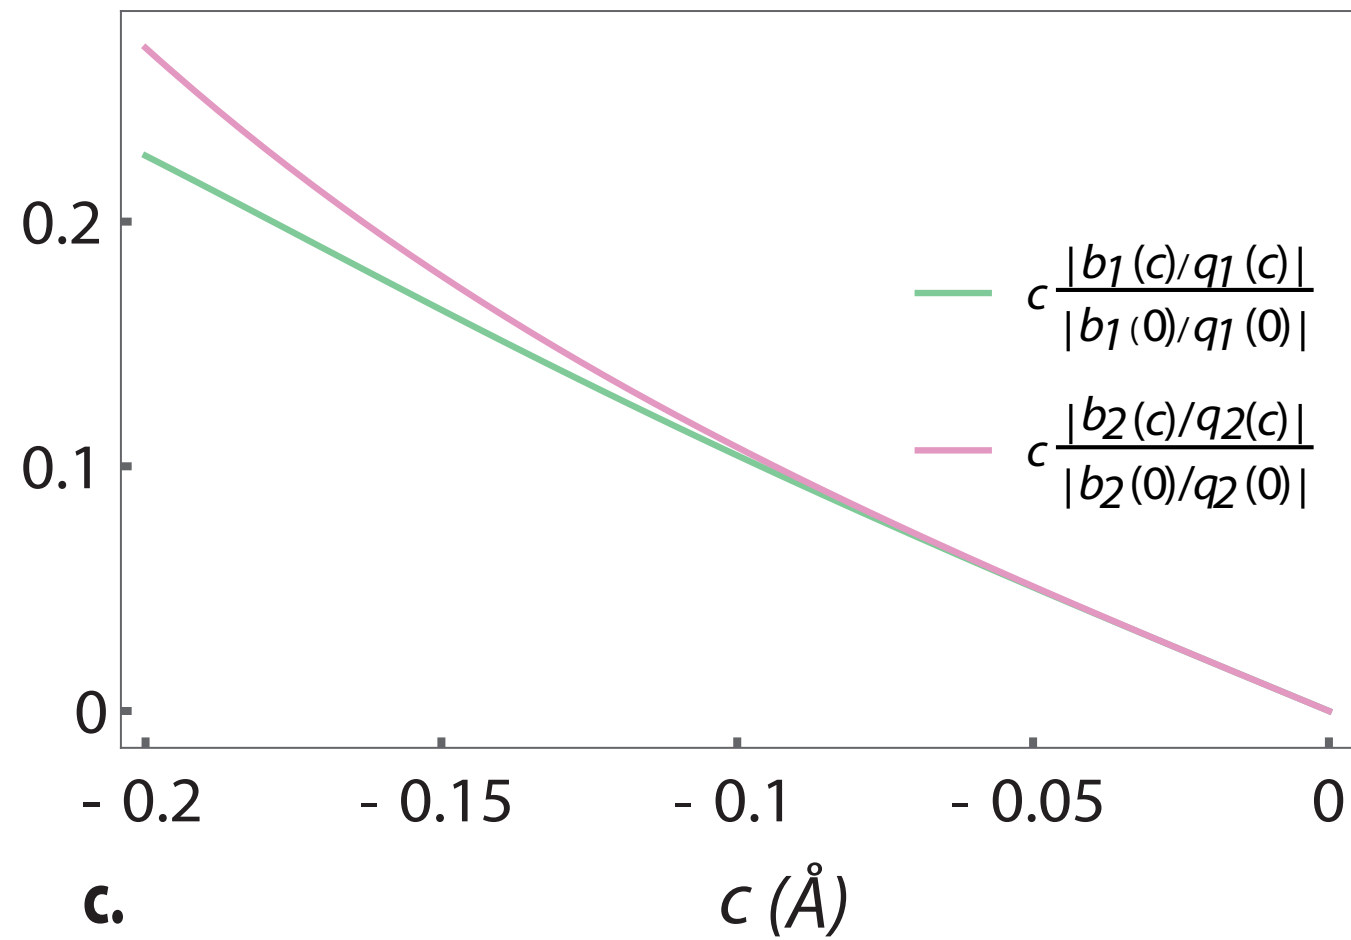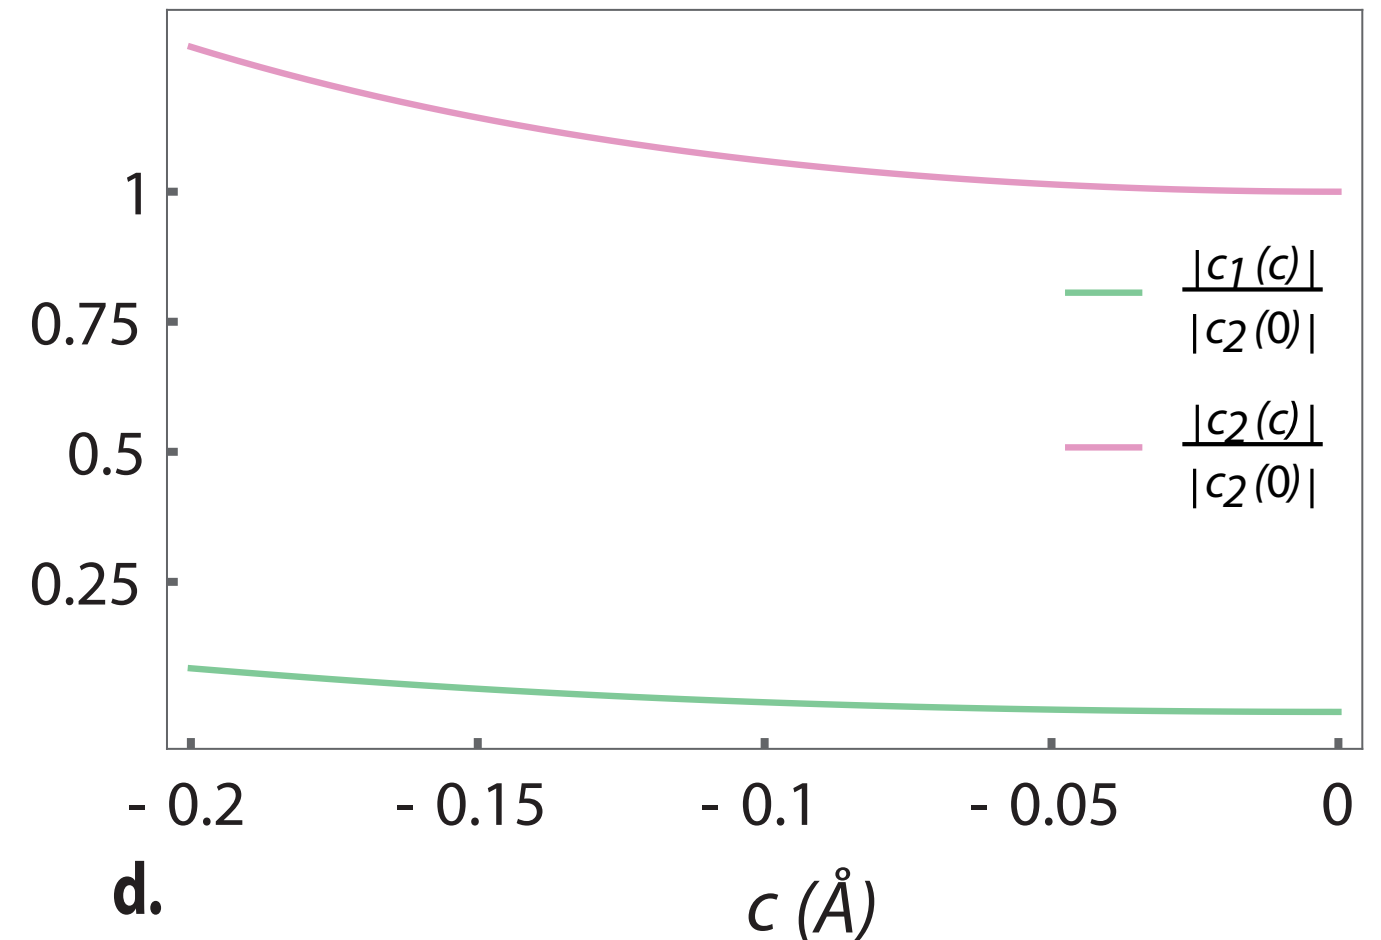

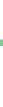

Supplement: Supplementary file 1 [file coeffappendicerev.pdf]
